# Supplementary material for: Learning Simple Algorithms from Examples
Source: arXiv:1511.07275 source file (2015-11-24)
Supplement: Supplementary file 1 [file supplementary.tex]

\section{Supplementary material}
We present few more experimental results that haven't fit into the main paper.


\subsection{Reward frequency vs reward reliability}
\label{subsec:freq}

Environment gives model reward, when model makes the correct prediction. However,
model can make a correct prediction for a wrong reason. For instance, 
model might pick a random number, and it happed to be correct. 
We can control this effect by manipulating base of operations (vocabulary size). For instance,
in base $2$ there are just $2$ possible answers either $0$ or $1$. Random 
guess would give a reward with probability $50\%$. 
Higher base means sparser reward, but more reliable. If you get it, then you are
likely to have it for the right reason.



Table \ref{tab:base}
presents median running time in minutes as base varies. Tasks like \textit{addition}, \textit{3 rows addition}
and \textit{single digit multiplication} are affected further on.
In case of this tasks, model has to memorize larger digit-to-digit operation table.
We have decided to present median running time, as success rate is so high that 
table becomes unreadable.



\input{"experiments/table_base.tex"}
\hline
\end{tabular}
\caption{Median running time over $10$ runs as we vary base (vocabulary size on different problems). It shows how important
is reward frequency versus it's reliability.}
\label{tab:base}
\end{table}



\subsection{Reward structure}
\label{subsec:reward}
\textbf{\underline{Notation}} \\
Let $y$ be the correct label, and
$p_i, i \in [0, 9]$ be a probability of predicting label $i$.

Reward in reinforcement learning systems drives learning process. 
In our setting, we control rewards, and decide when to give it. 
Our vanilla setting gives a rewards of $1$ for every correct prediction
, and reward $0$ for every incorrect one. Moreover, we terminate 
episode when system makes an incorrect prediction. We refer to this 
setting as ``0/1 reward''. We consider two other settings in addition to this. 

In setting ``Discretized reward''
, we sort $p_i$. That gives us an order on indices $a_1, a_2, \dots, a_10$,
i.e. $p_{a_1} \geq p_{a_2} \geq p_{a_3} \dots \geq p_{a_10}$.
We yield reward of $1$ iff $a_1 \equiv y$, reward of $\frac{1}{2}$ iff $a_2 \equiv y$,
and reward of $\frac{1}{3}$ iff $a_3 \equiv y$. Otherwise, we give a reward of $0$.


``Continuous reward'' setting gives a reward of $p_y$ for every prediction.
One could also consider reward $\log(p_y)$, however this quantity is unbouded,
and further processing might be necessary to make it work.

Table \ref{tab:more_reward} presents our experimental results.
We have expected that continuous reward would convey much more information than a discrete one. 
This should result in the better training.
However, results doesn't support this hypothesis. It seem to be even slightly harder to solve
problems with continuous reward than with a discrete one. However, this results might be
not statistically significant.
Continuous reward makes environment less stationary, which might make $Q$-learning
less efficient.



\input{"experiments/table_more_reward.tex"}
\hline
\end{tabular}
\caption{Figure compares results for different kinds of rewards. 
It presents median running time in minutes.
``0/1 reward'': model gets a reward of $1$ for every correct prediction, and $0$ otherwise. 
``Discretized reward'' provides few more values of reward prediction was sufficiently close to the
correct one. ``Continuous reward'' gives a probability of correct answer as the reward.}
\label{tab:more_reward}
\end{table}
